# Supplementary material for: The Multi-Temporal Urban Development SpaceNet Dataset
Source: arXiv:2102.04420 source file (2021-02-08)
Supplement: Supplementary file 1 [file sn7_v02_supplemental.tex]

Dataset histograms?
